# Supplementary material for: Condensed interior-point methods: porting reduced-space approaches on GPU hardware
Source: arXiv:2203.11875 source file (2022-03-22)
Supplement: Supplementary file 1 [file appendix.tex]

\subsection{Power flow model}
\subsubsection{Introducing the network model}
\label{sec:modeling:notations}
Let a power grid with $n_b$ buses, $n_g$ generators and $n_\ell$
lines. We denote by $\underline{\bm{v}}, \underline{\bm{I}} \in \mathbb{C}^{n_b}$
the bus voltage and current injections vectors, by $\underline{\bm{s}}_g \in \mathbb{C}^{n_g}$
the power generations and by $\underline{\bm{s}}_d \in \mathbb{C}^{n_b}$
the power loads at the different buses.
In polar notation, the bus voltage vector $\underline{\bm v}$ is decomposed
as $\underline{\bm v} = \bm{v}\,  e^{\underline{j} \bm{\theta}}$, with
$\bm{v}, \bm{\theta} \in \mathbb{R}^{n_b}$ the magnitude and the phase
of the complex voltage vector. Similarly, we decompose the power generations
$\underline{\bm{s}}^g = \bm{p}^g + \underline{j} \bm{q}^g$ into active
and reactive power generations $\bm{p}^g, \bm{q}^g \in \mathbb{R}^{n_g}$

\paragraph{Network's topology}
The power generated at the \emph{generators} is transmitted
through the \emph{lines} of the power network to
satisfy the demands at each \emph{bus}.
Hence, the topology of the network specifies
how the buses, the lines and the generators connect between each other.
The topology is usually given in the form of sparse connection matrices:
\begin{itemize}
  \item The \emph{generator-bus connection matrix} $C_g \in \mathbb{B}^{n_b \times n_g}$ connecting the generators to the buses;
  \item The \emph{from} and \emph{to} \emph{bus-line connection matrices} $C_f, C_t \in \mathbb{B}^{n_\ell \times n_b}$ associated to the standard $\pi$ transmission
    line model.
\end{itemize}
The values associated to the $\pi$ transmission line model
are given by four complex-valued vectors $Y_{ff}, Y_{ft}, Y_{tf}, Y_{tt}
\in \mathbb{C}^{n_\ell}$.
The system admittance matrices are then given as
\begin{equation}
  \begin{aligned}
    & Y_f = \diag{Y_{ff}} C_f + \diag{Y_{ft}} C_t \\
    & Y_t = \diag{Y_{tf}} C_f + \diag{Y_{tt}} C_t \\
    & Y_{bus} = C_f^\top Y_f + C_t^\top Y_t + \diag{Y_{sh}} \, .
  \end{aligned}
\end{equation}
The bus admittance matrix $\underline{Y}_{bus}$ is
usually decomposed into its conductance and its susceptance components $G, B \in \mathbb{R}^{n_b\times n_b}$:
$\underline{Y}_{bus} = G + \underline{j} B$
\subsubsection{Power flow equations}
The power injection vector $\underline{\bm{s}}^{inj} \in \mathbb{C}^{n_g}$ satisfies the Kirchhoff equation:
\begin{equation}
  \underline{\bm{s}}^{inj} = \underline{\bm{v}}\, \underline{\bm{I}}^*
  = \underline{\bm{v}} \,(Y_{bus}\, \underline{\bm v})^*
  \; .
\end{equation}
The power flow balance equations states that the power injections
$\underline{\bm s}^{inj}$ equates the difference between the power generations and the power loads,
with $\underline{\bm{s}}^{inj} = C_g \underline{\bm s}^g - \underline{\bm s}^d$.
By taking their real and imaginary parts, the $n_b$ complex power flow
equations decompose into $2 \times n_b$ real power flow equations,
writing for all buses $i = 1,\cdots,n_b$,
\begin{equation}
  \label{eq:powerflow}
  \left\{
  \begin{aligned}
    p_i^{inj} &= v_i \sum_{j =1}^{n_b} v_j (g_{ij}\cos{(\theta_i - \theta_j)} + b_{ij}\sin{(\theta_i - \theta_j})) \,,  \\
    q_i^{inj} &= v_i \sum_{j = 1}^{n_b} v_j (g_{ij}\sin{(\theta_i - \theta_j)} - b_{ij}\cos{(\theta_i - \theta_j})) \,.
  \end{aligned}
  \right.
\end{equation}
We note that in~\eqref{eq:powerflow}, the power injection depends only on
the voltage magnitudes $\bm{v}$ and the voltage angles $\bm{\theta}$.
We rewrite the power flow in vector notation with the functional
$G: \mathbb{R}^{n_b} \times \mathbb{R}^{n_b} \times \mathbb{R}^{n_g} \times \mathbb{R}^{n_g} \to
\mathbb{R}^{2n_b}$, as
\begin{equation}
  \label{eq:powerflowvec}
  G(\bm{v}, \bm{\theta}, \bm p^g, \bm q^g) =
    \begin{bmatrix}
      \bm{p}^{inj}(\bm{v}, \bm{\theta}) - C_g \bm{p}^{g} + \bm{p}^d \\
      \bm{q}^{inj}(\bm{v}, \bm{\theta}) - C_g \bm{q}^{g} + \bm{q}^d
    \end{bmatrix}
    = 0 \; .
\end{equation}

\paragraph{Line flow limits}
The amount of power transiting through the transmission lines is limited by the thermal
limits. The complex power injections at the \emph{from} and the \emph{to} ends of all lines
are given by
\begin{equation}
  \label{eq:power_inj_line}
  \underline{\bm{s}}_f = \diag{C_f \underline{\bm{v}}} \; \underline{Y_f} \underline{\bm{v}} \; , \quad
  \underline{\bm{s}}_t = \diag{C_t \underline{\bm{v}}} \; \underline{Y_t} \underline{\bm{v}} \;
  \; ,
\end{equation}
In \eqref{eq:power_inj_line}, the power injections depend only
on the voltage magnitudes and angles $\bm v, \bm \theta$.
The thermal limits are bounded by a vector $F^{\sharp}_\ell \in \mathbb{R}^{n_\ell}$.
We define the line limits with a functional $H: \mathbb{R}^{n_b} \times \mathbb{R}^{n_b} \to
\mathbb{R}^{2 n_\ell}$, such as
\begin{equation}
  H(\bm v, \bm \theta) = \begin{bmatrix}
    \underline{\bm s}_f (\underline{\bm s}_f)^* \\
    \underline{\bm s}_t (\underline{\bm s}_t)^*
  \end{bmatrix}
  \leq
  \begin{bmatrix}
    (F_\ell^{\sharp})^2 \\
    (F_\ell^{\sharp})^2
  \end{bmatrix}
  \; ~
  (= \bm{h}^\sharp)
  \; .
\end{equation}

The power flow balances are defined as
\begin{equation}
  \label{eq:base:powerflow}
  G(\bm v, \bm \theta, \bm p^g, \bm q^g) =
  \overbrace{
  \begin{bmatrix}
    G^c & B^s & G^d\\
    -B^c & G^s & -B^d
  \end{bmatrix}
  }^{M}
  \psi(\bm v, \bm \theta)
  +
  \begin{bmatrix}
    \bm{p}^d - C_g \bm{p}^g \\
    \bm{q}^d - C_g \bm{q}^g
  \end{bmatrix}
\end{equation}
with $C_g$ the generator-bus incidence matrix, $G^{c,s,d}, B^{c,s,d}$ subsets
of the conductance and susceptance matrices.
The powers transiting on the lines of the network satisfy
\begin{equation}
  \label{eq:base:powerlines}
    \begin{bmatrix}
    \bm s_p^f \\ \bm s_q^f
    \end{bmatrix}
    =
    \overbrace{
    \begin{bmatrix}
    G_{ft} & B_{ft} & G_{ff} C_f^\top \\
    -B_{ft} & G_{ft} & -B_{ff} C_f^\top
    \end{bmatrix}
    }^{L_{line}^f}
    \psi(\bm v, \bm \theta)
    \; , \quad
    \begin{bmatrix}
    \bm s_p^t \\ \bm s_q^t
    \end{bmatrix}
    =
    \overbrace{
    \begin{bmatrix}
    G_{tf} & B_{tf} & G_{tt} C_t^\top \\
    -B_{tf} & G_{tf} & -B_{tt} C_t^\top
    \end{bmatrix}
    }^{L_{line}^t}
    \psi(\bm v, \bm \theta)
\end{equation}
We define the line limits with a functional $H: \mathbb{R}^{n_b} \times \mathbb{R}^{n_b} \to
\mathbb{R}^{2 n_\ell}$ such as
\begin{equation}
  \label{eq:linelimitsvec}
  H(\bm v, \bm \theta) = \begin{bmatrix}
    (\bm s_p^f)^2 + (\bm s_q^f)^2 \\
    (\bm s_p^t)^2 + (\bm s_q^t)^2
  \end{bmatrix}
  \leq
  \begin{bmatrix}
    (F_\ell^{\sharp})^2 \\
    (F_\ell^{\sharp})^2
  \end{bmatrix}
  \; ~
  (= \bm{h}^\sharp)
  \; .
\end{equation}
\end{subequations}
We note that once the basis $\psi(\bm v, \bm \theta)$ is computed,
evaluating \eqref{eq:base:powerflow} and \eqref{eq:base:powerlines}
involves only sparse matrix-vector product operations ({\tt SpMV})
with the three sparse matrices $M, L_{line}^f$ and $L_{line}^t$
as well as with the incidence matrices $C_g, C_f, C_t$.
The cosine and the sine terms are evaluated only once, and then reused
throughout the different computations.

\paragraph{Optimal power flow problem.}
We get the ACOPF problem written in polar form:
\begin{subequations}
  \label{eq:acopf}
  \begin{align}
      \label{eq:acopf:obj}
      \min_{\bm{v}, \bm{\theta}, \bm{p}, \bm{g}} & \; \sum_{i=1}^{n_g} c^g_{i,1} (p_i)^2 + c_{i,2}^g (p_i) + c_{i, 3}^g \\
      \label{eq:acopf:cons}
      \text{subject to } ~ & G(\bm{v}, \bm{\theta}, \bm p, \bm q) = 0 \, \quad  H(\bm v, \bm \theta) \leq \bm{h}^\sharp \, , \\
      \label{eq:acopf:bounds1}
                           & \bm{v}^\flat \leq \bm{v} \leq \bm{v}^\sharp\, , \quad \theta_{ref} = 0 \; , \\
      \label{eq:acopf:bounds2}
                    & \bm{p}^\flat \leq \bm{p}^g \leq \bm{p}^\sharp \; , ~ \bm{q}^\flat \leq \bm{q}^g \leq \bm{q}^\sharp \; .
  \end{align}
\end{subequations}
The quadratic objective~\eqref{eq:acopf:obj} depends only on the active power generation,
with the cost coefficients $c^g_1, c^g_2, c^g_3 \in \mathbb{R}^{n_g}$.
In~\eqref{eq:acopf:cons}, the equality constraint $G$ encodes the $2\times n_b$ complete power balance equations
and the inequality constraint $H$ encodes the $2 \times n_\ell$ line flow limits.
The bounds~\eqref{eq:acopf:bounds1}-\eqref{eq:acopf:bounds2}
ensure that the voltage magnitudes and the power generations satisfy their operational limits.

\paragraph{Reduced space problem}
We are now able to exploit the structure of the powerflow
manifold~\eqref{eq:powerflowreduced} to remove all the state
variables form the optimal power flow problem, reducing by
$n_x$ the total dimension of the OPF problem~\eqref{eq:acopf}.
Formally, this is a consequence of the implicit function theorem.

Hence, we can derive a new OPF formulation depending only
on the control $\bm u$. To do that, we first rewrite
the original ACOPF problem \eqref{eq:acopf} with the state $\bm x$
and the control $\bm u$ as optimization variables.
First, the line flow constraints rewrite directly as
\begin{equation}
  h(\bm x, \bm u) := H(\bm v, \bm \theta)  \; .
\end{equation}
Second, unlike to the original ACOPF problem~\eqref{eq:acopf},
the active power generation at the slack bus and the reactive power
generations are only considered \emph{implicitly}, with
\eqref{eq:powerflowineq}. Hence, we have to introduce
additional nonlinear constraints to amount for the bounds on the
active and reactive power generations. We denote a
new set of constraints by the function $r:\mathbb{R}^{n_x} \times \mathbb{R}^{n_u}
\to \mathbb{R}^{n_{ref} + n_{gen}}$, defined as
\begin{equation}
  \label{eq:implicitcons}
  \overbrace{
  \begin{bmatrix}
    C_{g,ref} \bm{p}^{g,\flat} \\
    C_{g,ref} \bm{q}^{g,\flat} \\
    C_{g,pv} \bm{q}^{g,\flat}
  \end{bmatrix}
  }^{\bm{r}^\flat}
  \leq
  \overbrace{
  \begin{bmatrix}
    \bm{p}^{inj}_{ref}(\bm v, \bm \theta) \\
    \bm{q}^{inj}_{ref}(\bm v, \bm \theta) \\
    \bm{q}^{inj}_{pv}(\bm v, \bm \theta)
  \end{bmatrix}
  }^{r(\bm x, \bm u)}
  \leq
  \overbrace{
  \begin{bmatrix}
    C_{g,ref} \bm{p}^{g,\sharp} \\
    C_{g,ref} \bm{q}^{g,\sharp} \\
    C_{g,pv} \bm{q}^{g,\sharp}
  \end{bmatrix}
  }^{\bm{r}^\sharp}
\end{equation}
We highly emphasize that when we define the implicit
mapping for the reactive power generations, we are \emph{de facto}
aggregating the reactive power generations on the PV buses.
If we have multiple generators associated to the same PV bus, we cannot recover
the individual reactive power generations for each generator.
In other words, we are \emph{losing} information if we have multiple
generators per bus, hence we are losing the equivalence with relation
to the original problem~\eqref{eq:acopf}.
\begin{equation}
  \label{eq:acopf_controlstate}
  \begin{aligned}
    \min_{\bm x, \bm u} \quad & f(\bm x, \bm u)                                            \\
    \text{subject to} \quad   & \bm{u}^\flat \leq \bm{u} \leq \bm{u}^\sharp  \;, \quad
\bm{x}^\flat \leq \bm{x} \leq \bm{x}^\sharp  \;, \\
                              & g(\bm x, \bm u) = 0 \; , \\
                              &\bm{r}^\flat \leq r(\bm x, \bm u) \leq \bm{r}^\sharp \; , \quad
                              h(\bm x, \bm u) \leq \bm{h}^\sharp \; .
  \end{aligned}
\end{equation}

\subsection{Reduction algorithm on GPU}
\subsection{Solving the OPF on GPU}
